# Supplementary material for: Voyager 2 solar plasma and magnetic field spectral analysis for intermediate data sparsity
Source: arXiv:1510.04304 source file (2015-08-24)
Supplement: Supplementary file 1 [file voy2_jgr_SI_14aug_2col.pdf]

# Supporting Information for "Voyager 2 solar plasma and magnetic field spectral analysis for intermediate data sparsity"

L. Gallana,[1] F. Fraternale,[1] S. M. Fosson,[2] E. Magli,[2] M. Opher,[3] J. D. Richardson,[4] , M. Iovieno[1], and D. Tordella[1]

**Contents of this file**

1. Fortran routine for the generation of synthetic datasets
2. Fortran routine for data interpolation and computation of the two-points correlations
3. Fortran routines for computation of power spectra
4. Fortran routines for averaged spectra from data subsets
5. Fortran routines for the maximum likelihood recovery
6. Matlab script for compress sensing spectral estimation
7. Comparison of the methods on V2 solar wind data

**Introduction**

This supporting information document is to give information about the software we use for the spectral estimation from gapped Voyager datasets. All the software is made of Fortran90 routines, except the *compressed sensing* method whic is implemented in the Matlab environment (the complete script is reported below). All the Fortran routines can be downloaded from our research group website `http://areeweb.polito.it/ricerca/philofluidsoftware.html`, where one can also find detailed instruction for the use of the codes. In the following we report a list of the routines and a brief describtion.

**Fortran routine for the generation of synthetic datasets**

This code can be used to generate synthetic turbulence datasets from imposed spectral properties. Uniformly distributed random phases are chosen before the inverse transform operation is performed. The code makes use of the C06GBF, C06FBF, C06FAF routines from the NAG library (not open-source). Another small Fortran routine is provided to project the same gap distribution of the Voyagers data onto the synthetic sequences.

**Fortran routine for data interpolation and computation of the two-points correlations**

This code reads the plasma and magnetic field data, computes average quantities, magnetic field in Alfvén variables and average plasma parameters. Following, the two-point correlation functions are computed, after linear interpolation of the data on a uniform time grid with the same $\Delta t$ as the spacecraft data. A subroutine is dedicated to find the best alignment with the original points in order to reduce errors when spectra are computed. The full correlation tensors can be computed (autocorrelations and cross correlations of velocity and magnetic field). To deal with large data sets, this code can be used with multiple threads by the *OpenMP* interface.

**Fortran routines for computation of power spectra**

This routines compute the power spectral density (PSD) of all the field components either from the correlation functions or directly from reconstructed datasets. The codes use the dffti, dfftf, dfftb routines from the FFTPack libraries (open source, see `http://www.netlib.org/fftpack/` for further details). Different subroutines are also included for spectral smoothing.

**Fortran routines for averaged spectra from data subsets**

This code can be used to compute averaged spectra. From the total period analyzed, different "continuous" subsets are identified. A continuous subset is defined as a sequence of data containing gaps below a certain threshold (called $T_g$, see the main text), which is an input parameter of the code. Given this threshold, the number of continuous subsets is uniquely identified. These sequences are linearly interpolated (if $T_g > \Delta t_{sampling}$) on a uniform time grid and the Fourier transform is computed. Before the FFT is performed, some techniques may be applied, such as data windowing (Hann or Welch windows) or detrending. All the computed spectra are then averaged. The codes use the dffti, dfftf, dfftb routines from the FFTPack libraries.

**Fortran routines for the maximum likelihood recovery** This set of five routines implement the maximum likelihood recovery method published by Rybicki &Press (1982). This code is derived from routines published on their webpage `http://www.lanl.gov/DLDSTP/fast/` which we modified to apply to the Voyager solar wind datas. The method reconstructs the data with a minimum variance recovery plus a stochastic component. So, the resulting reconstruction is constrained by the data where the data are present, while it is stochastic in the gaps, with the same second order statistical properties of the data. Since the recovery is not deterministic, different realizations can be obtained. The reconstruction is based on a correlation function, which has to be given as an input. We use the correlation function $\rho(\tau)$ computed from linearly interpolated data. Since the code involves operations such as eigenvalue/eigenvector computation of the correlation matrix, as well as matrix inversions, the correlation function has to be quite smooth. This requirement holds for lag times $\tau$ below a certain threshold $\tau_{max}$ so only data segments of size below $\tau_{max}$ can be recovered at a time. For this reason the input dataset is split into subsets. Since usually the biggest gap is shorter than $\tau_{max}$, the entire dataset can be reconstructed. The user can choose to recover the global dataset or only some subset of it. Parameters of the code are related to the segmentation, for the details we refer to the software user guide in our group webpage. This code uses the DSYSV, DGEMV, DSYTRF, DSYTRI routines from the LAPACK libraries (open source).

[1]Dipartimento di Ingegneria Meccanica e Aerospaziale, Politecnico di Torino, Torino, Italy.
[2]Dipartimento di Elettronica e Telecomunicazioni, Politecnico di Torino, Torino, Italy.
[3]Astronomy Department, Boston University, Boston, MA, USA
[4]Kavli Institute for Astrophysics and Space Research, Massachusetts Institute of Technology (MIT), Cambridge, MA, USA

Copyright 2015 by the American Geophysical Union.
0148-0227/15/$9.00

**Matlab script for compressed sensing spectral estimation**

The following Matlab script implements the *compressed sensing* algorithm for the power spectrum estimation. The numerical solution is obtained by the SPGL1 solver (`https://www.math.ucdavis.edu/~mpf/spgl1/`) in the Fourier framework. This script is for a three-components field.

```
clear all
close all
clc

%addpath spgl1-1.8/
dd=load('dati_U_hires_2008.0_2008.2.txt');
% file format: [time(s), U1, U2, U2]
tot_run=1; % =n splits the data in n segments
 and computes averaged output
sigma=0.01;% noise parameter for bpdn
step=192;  % data sampling time (sec)

nn=size(dd,1); % change nn if you want to
%read only the first nn point of file

d(:,1)=dd(1:nn,1)- dd(1,1);
d(:,2)=dd(1:nn,2)-mean( dd(1:nn,2) );
d(:,3)=dd(1:nn,3)-mean( dd(1:nn,3) );
d(:,4)=dd(1:nn,4)-mean( dd(1:nn,4) );

time=zeros(1,size(d,1));
time(1)=1;
for h=2:nn
gap(h-1)=round((d(h,1)-d(h-1,1))/step);
time(h)=time(h-1)+gap(h-1);
end

L=floor((floor(max(time)/tot_run))/2)*2
% L must be even
Vr=zeros(L/2, tot_run);
Vt=zeros(L/2, tot_run);
Vn=zeros(L/2, tot_run);

Vr_recovered=zeros(L, tot_run);

K=zeros(tot_run,1);
for run=1:tot_run
disp(run);
[~,ei]=min(abs(time-(L*(run-1)+1)));
[~,es]=min(abs(time-run*L));
window=[ei:es];
r=time(window)-time(window(1))+1;
K(run)=length(window);

% BASIS PURSUIT DENOISE

opA = @(x,mode) partialFourier(r,L,x,mode);
% This is now "A"
opts = spgSetParms('verbosity',0);
z = spg_bpdn(opA,d(window,2),sigma, opts);
% if one want to use bp instead of bpdn
       %z = spg_bp(opA,d(window,2), opts);
       % power spectrum
Vr(:,run)=K(run)*step*(abs(z(1:L/2))).^2;
z =  spg_bpdn(opA,d(window,3),sigma, opts);
%to check the correct recovery of input points
        inverset2=ifft(z)*sqrt(L);
        inverset1=partialFourier(r,L,z,1);
Vt(:,run)=K(run)*step*(abs(z(1:L/2))).^2;
z =  spg_bpdn(opA,d(window,4),sigma, opts);
Vn(:,run)=K(run)*step*(abs(z(1:L/2))).^2;
clear r

end

figure(1),hold on
plot(time(1:end),inverset1,'ob')
plot(time(1:end),d(:,3),'+r')
plot(time(end):-1:1,inverset2,'+c')

f=[1:L/2]'/(step*L)        %frequencies
Vr_mean=sum(Vr,2)/sum(K);
Vt_mean=sum(Vt,2)/sum(K);
Vn_mean=sum(Vn,2)/sum(K);
BP=[f, 2*Vr_mean, 2*Vt_mean, 2*Vn_mean, ...
2*(Vr_mean+Vt_mean+Vn_mean)];

%save('OUTPUT_CS.txt','BP', '-ascii');
figure(2)
loglog(BP(:,1), BP(:,5),'*r')
xlabel('f (Hz)');
ylabel('PSD |U|');
```

**Comparison of the methods on V2 solar wind data**

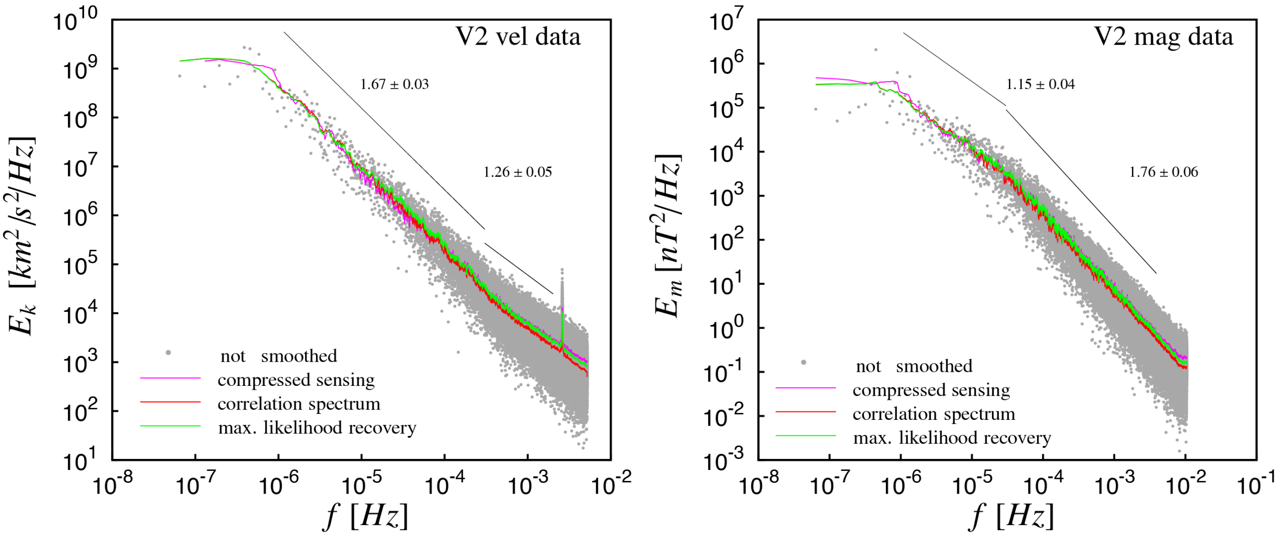


**Figure S1.** Kinetic (left) and magnetic (right) energy spectra for Voyager 2 data in the period 1979, DOY 1-180 (5 AU, close to the ecliptic). Here three methods of analysis are compared. *Pink:* compressed sensing; *red:* correlation spectrum after linear interpolation of the data; *green:* spectrum of the maximum likelihood recovery. In the case of about 30% of data are missing, and the three techniques lead to very similar results. The maximum difference in the slopes is around 4%. To show this, a smoothing has been applied to the spectra. The grey points represent the not-smoothed correlation spectra.
